# Supplementary material for: LEGO: Leveraging Experience in Roadmap Generation for Sampling-Based Planning
Source: arXiv:1907.09574 source file (2019-07-22)
Supplement: Supplementary file 1 [file suppl_experiment_results.tex]

% !TEX root = ../supplementary.tex

\begin{figure*}[!ht]
\centering
%%%%%%%%%%%%%%%%%%%%%%%%%%%%%%% 2D POINT ROBOT
  \begin{subfigure}[b]{0.27\textwidth}
    \centering
    \includegraphics[height=10.70em]{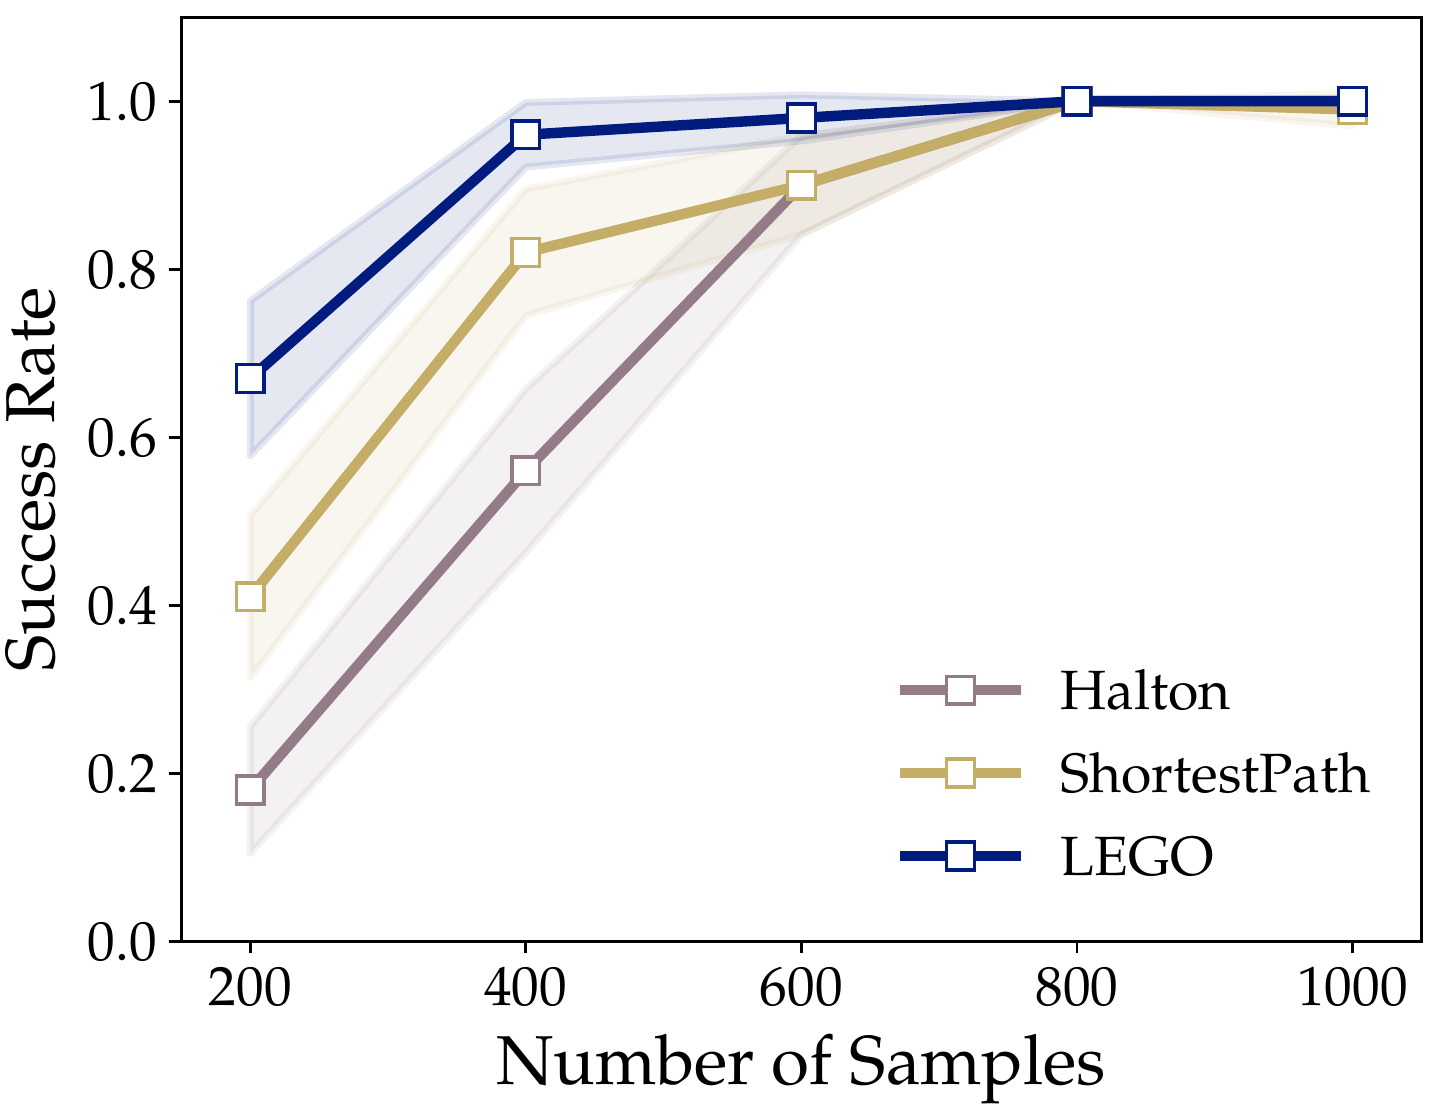}
    \caption{}
    \label{fig:4_2D_sr}
    \vspace*{1em}
  \end{subfigure}
  \begin{subfigure}[b]{0.27\textwidth}
    \centering
    \includegraphics[height=10.70em]{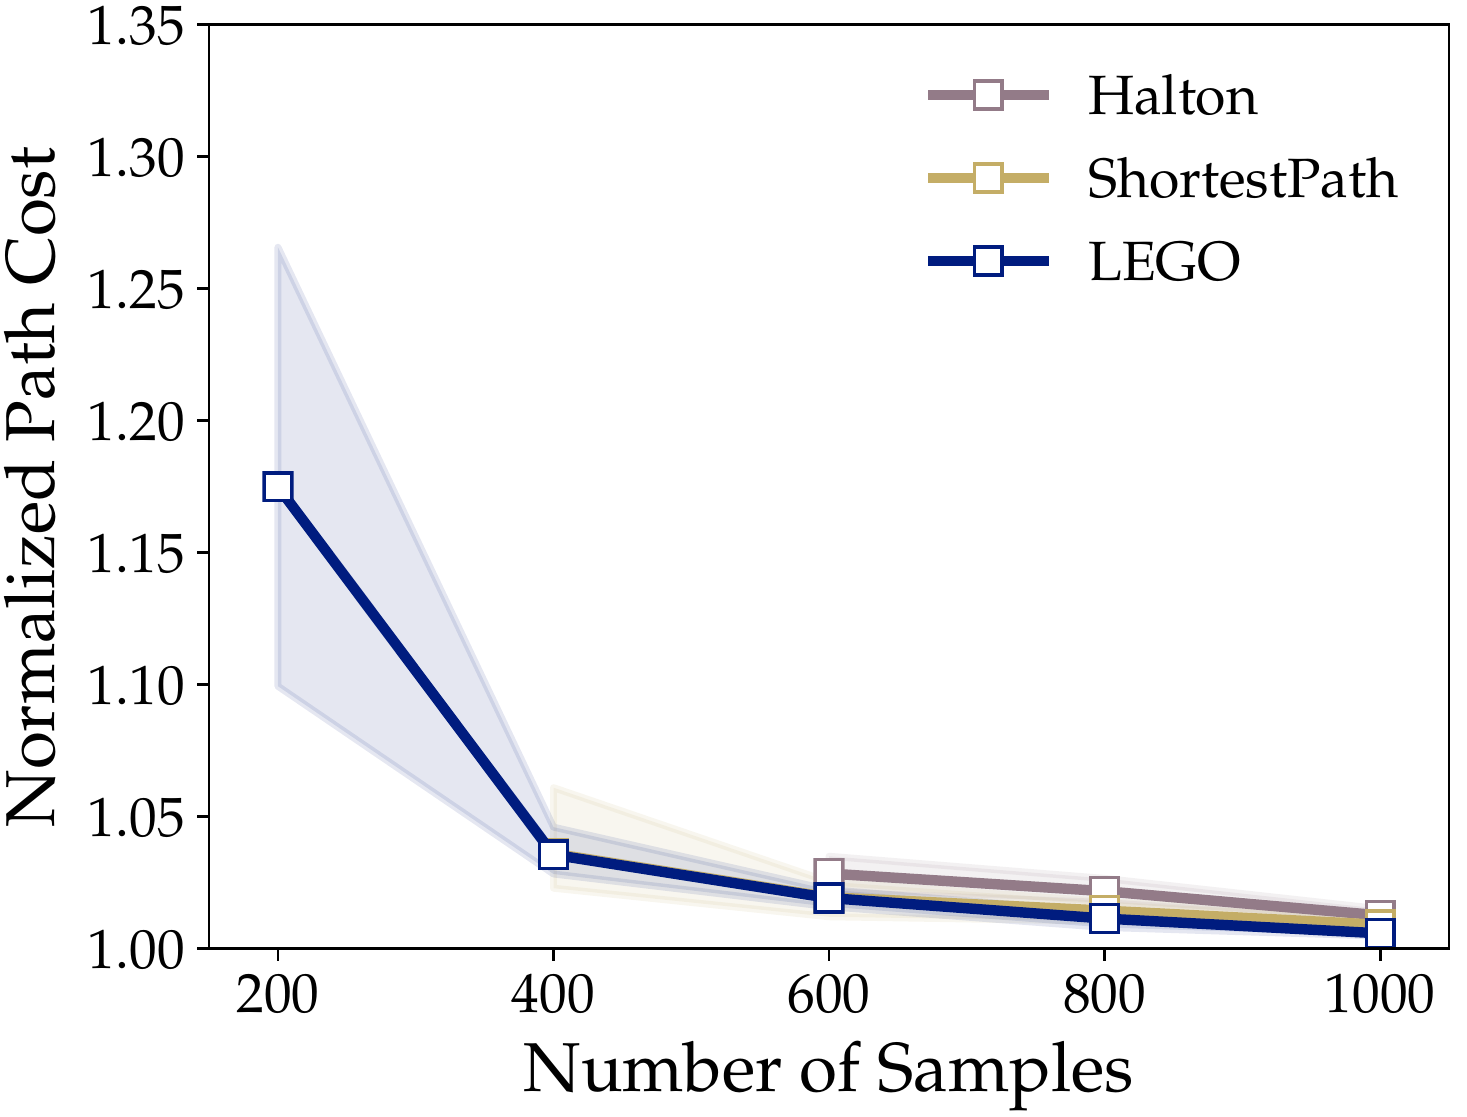}
    \caption{}
    \label{fig:4_2D_pl}     
    \vspace*{1em}
  \end{subfigure}
  \begin{subfigure}[b]{0.21\textwidth}
    \centering
    \includegraphics[height=10.75em]{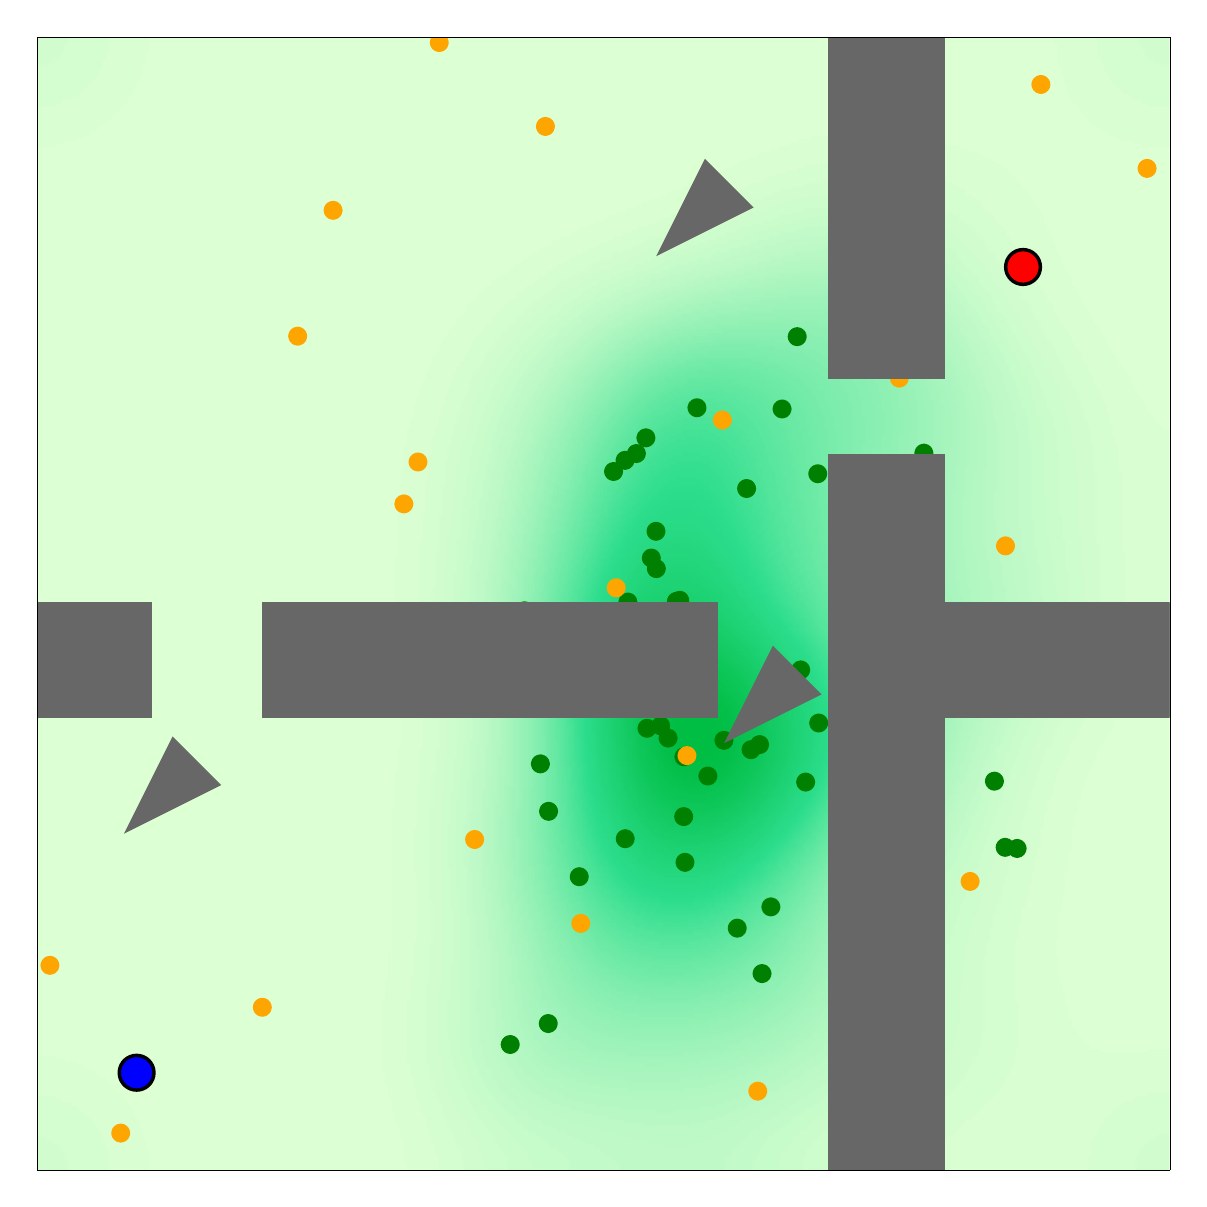}
    \caption{}
    \label{fig:4_2D_sp}     
    \vspace*{1em}
  \end{subfigure}
  \begin{subfigure}[b]{0.21\textwidth}
    \centering
    \includegraphics[height=10.75em]{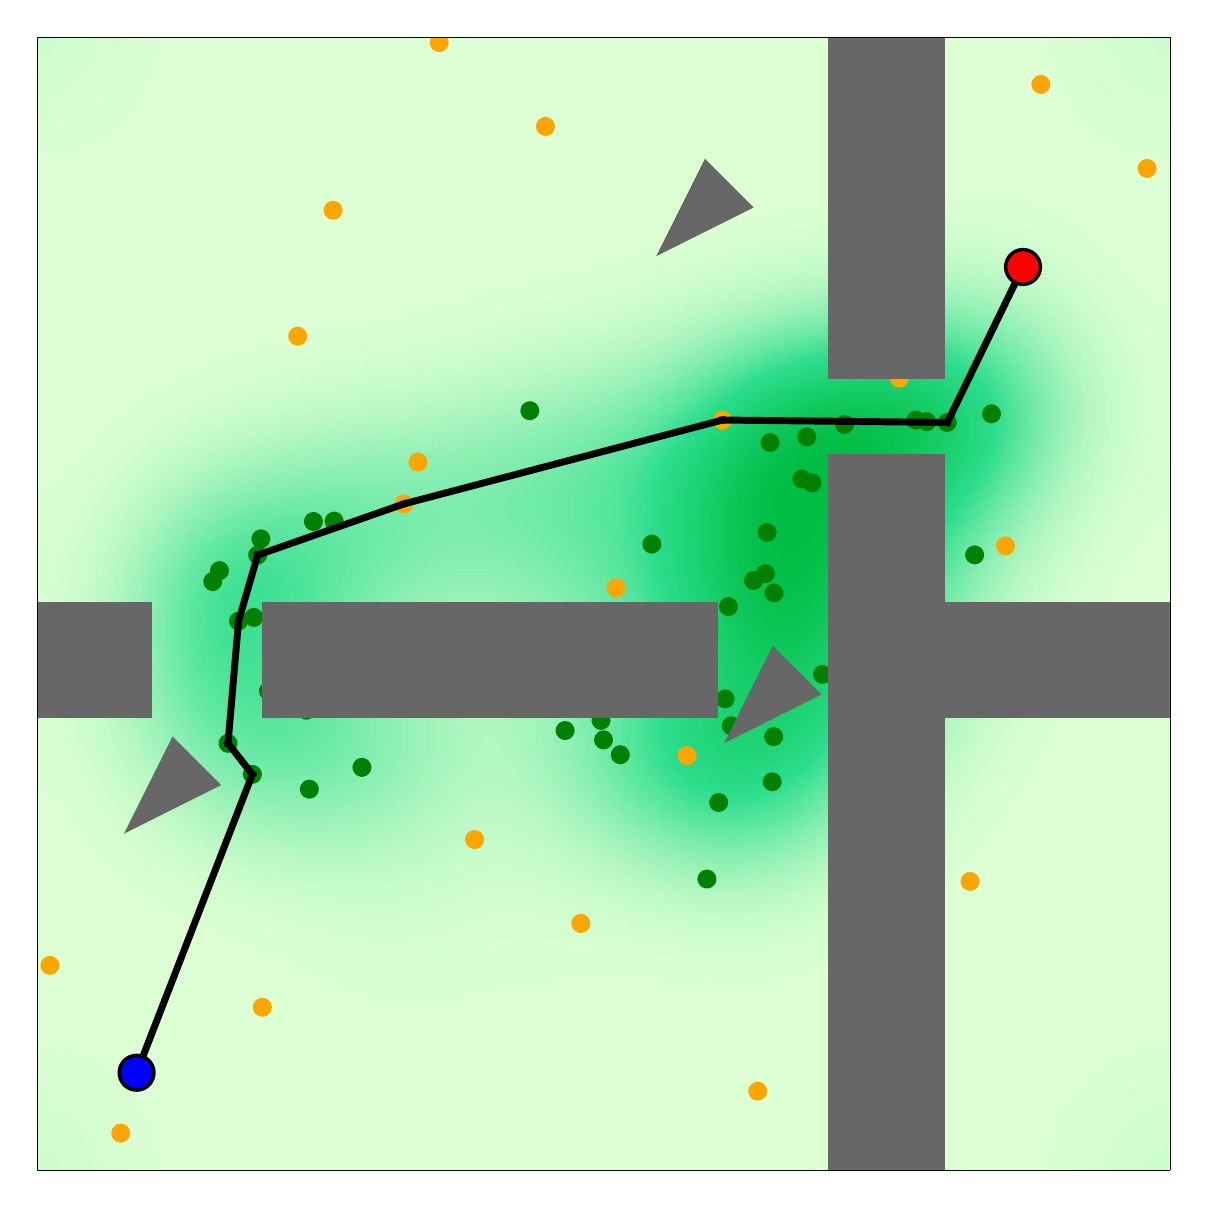}
    \caption{}
    \label{fig:4_2D_lego}     
    \vspace*{1em}
  \end{subfigure}
%%%%%%%%%%%%%%%%%%%%%%%%%%%%%%% 5D SNAKE
  \begin{subfigure}[b]{0.27\textwidth}
    \centering
    % \framebox[\linewidth]{\raisebox{0pt}[0.7\linewidth][0pt]{{\large Snake}}}
    \includegraphics[height=10.70em]{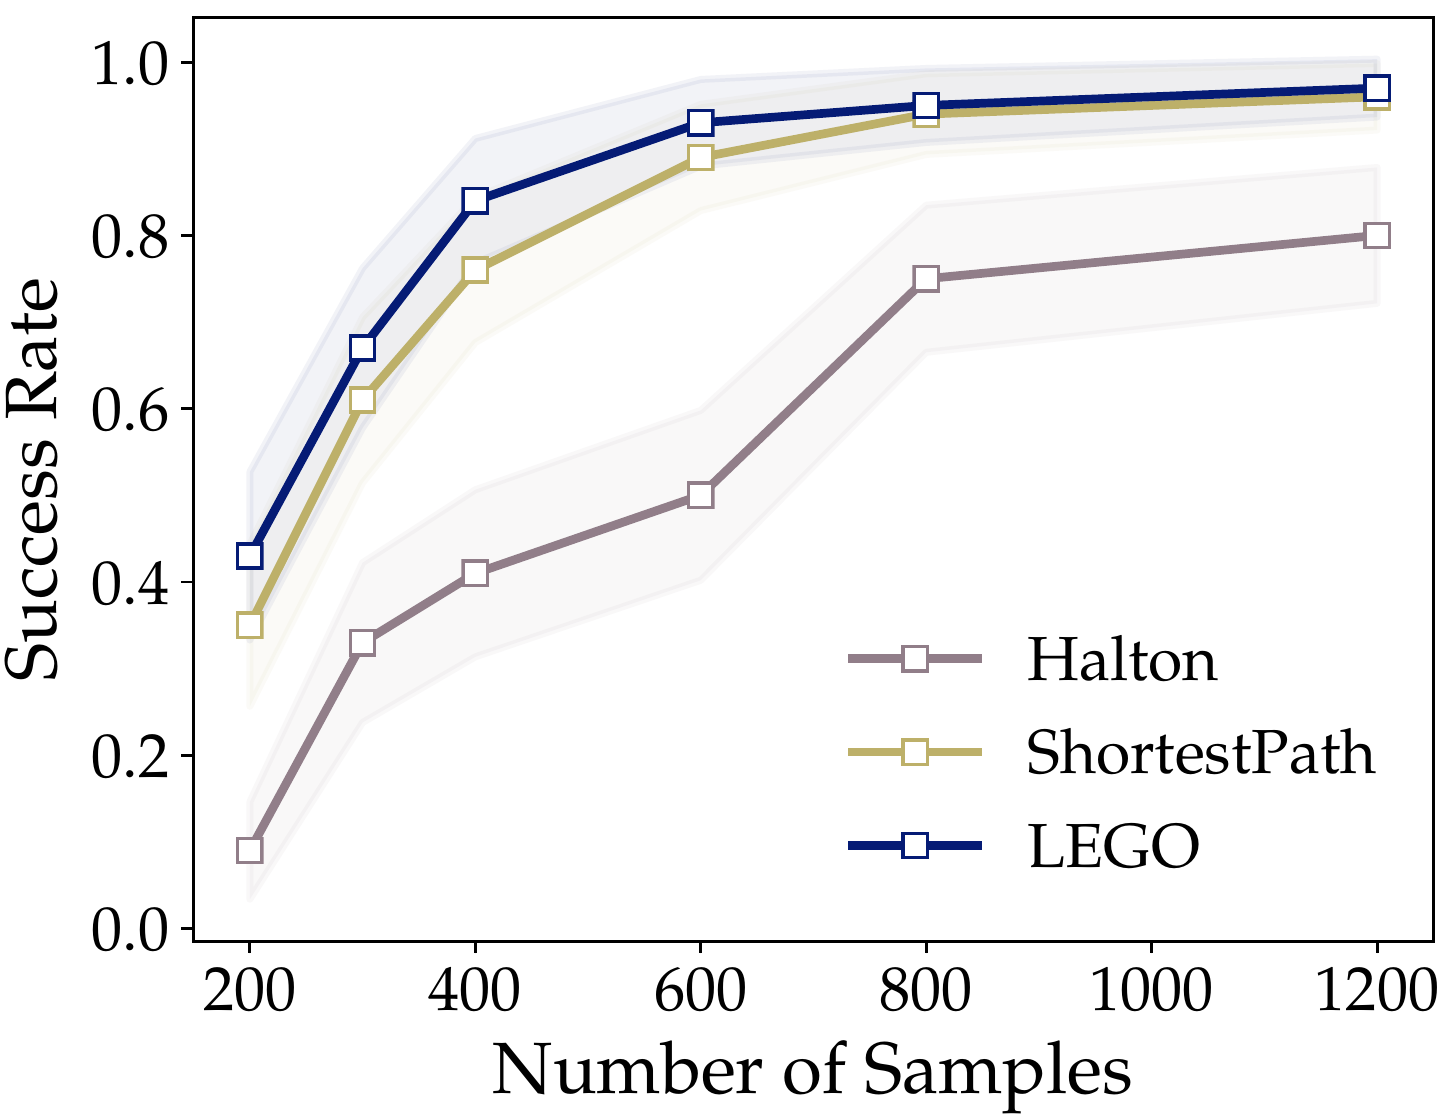}
    \caption{}
    \label{fig:4_3D_sr}
    \vspace*{1em}
  \end{subfigure}
  \begin{subfigure}[b]{0.27\textwidth}
    \centering
    % \framebox[\linewidth]{\raisebox{0pt}[0.7\linewidth][0pt]{{\large Snake}}}
    \includegraphics[height=10.70em]{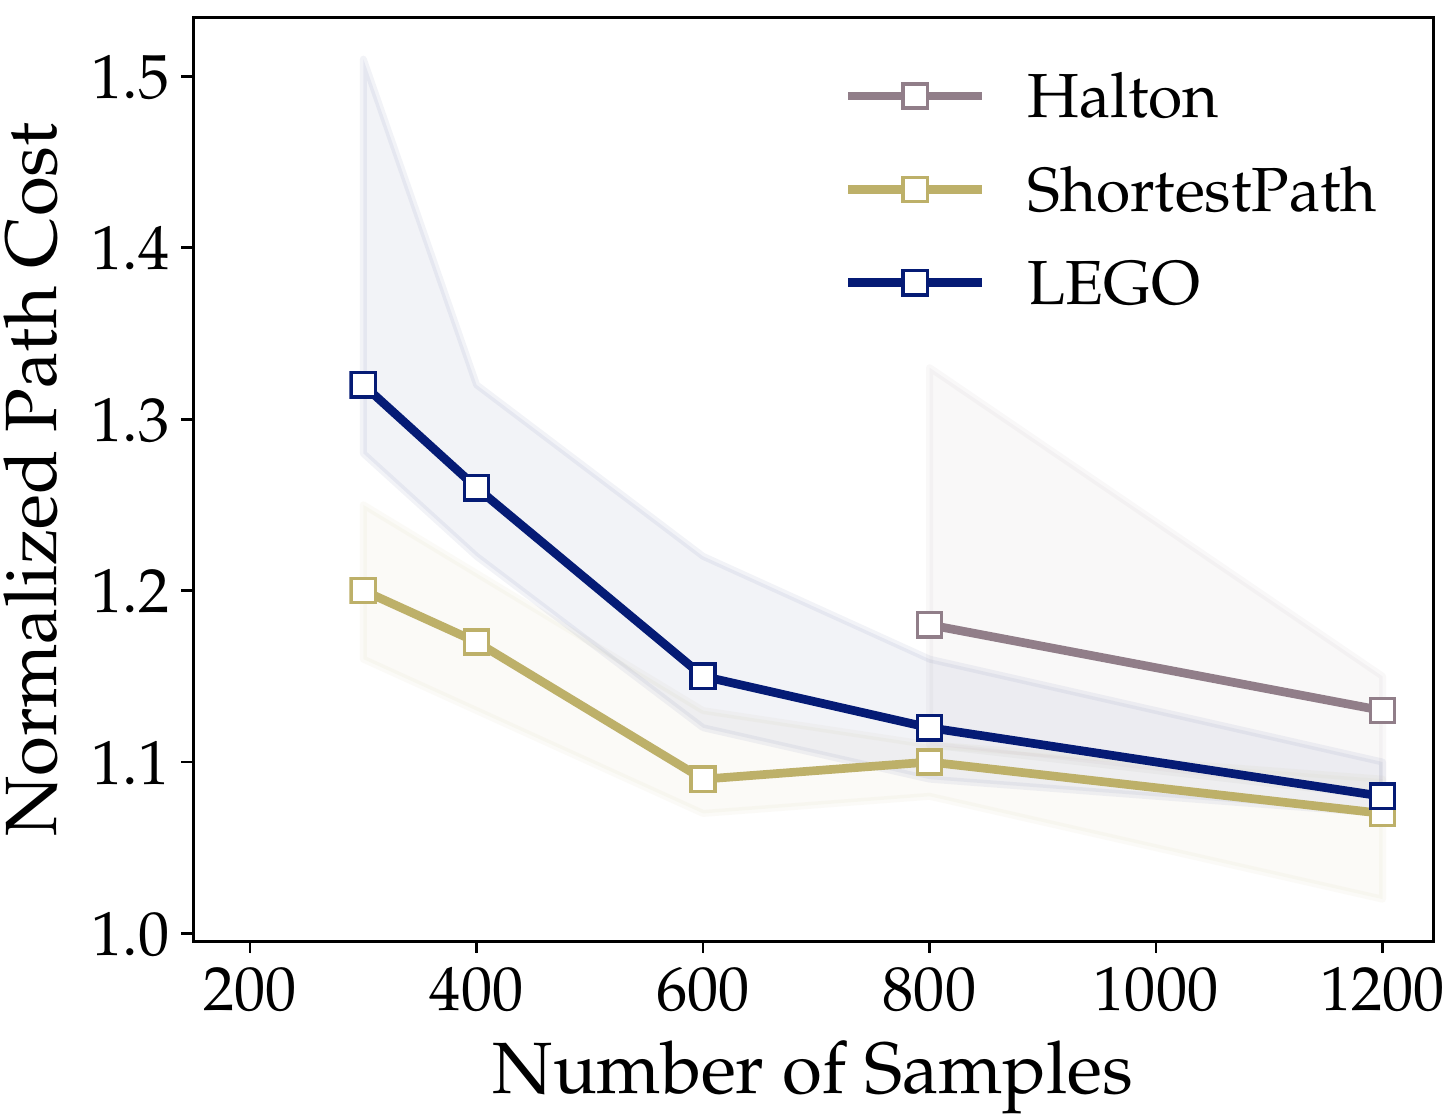}
    \caption{}
    \label{fig:4_3D_pl}
    \vspace*{1em}
  \end{subfigure}
  \begin{subfigure}[b]{0.21\textwidth}
    \centering
    \includegraphics[height=10.75em]{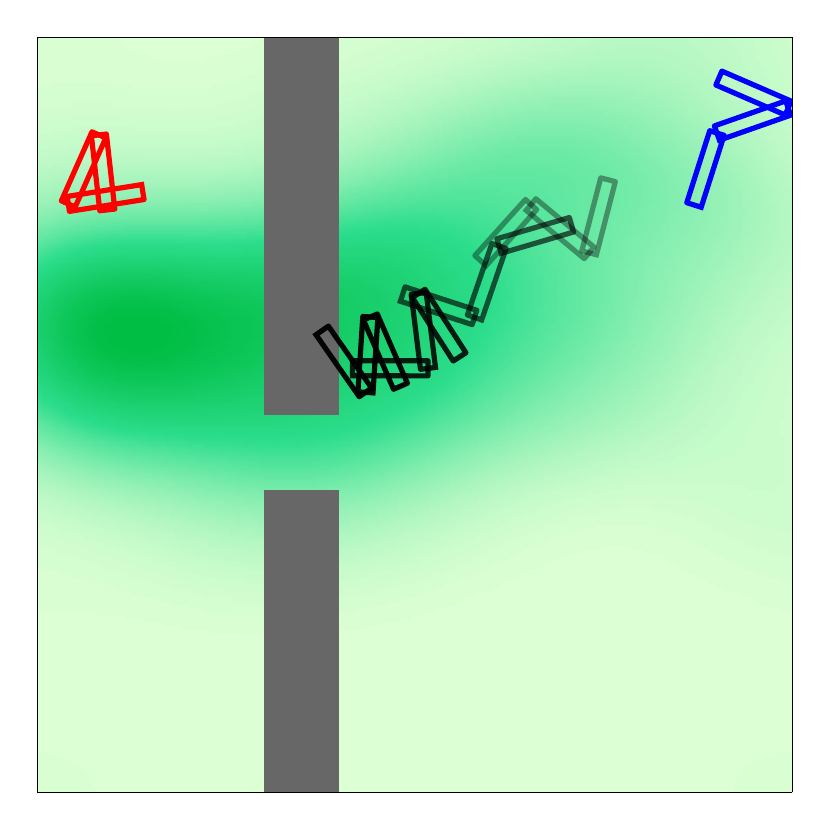}
    % \framebox[\linewidth]{\raisebox{0pt}[0.7\linewidth][0pt]{{\large Snake}}}
    \caption{}
    \label{fig:4_3D_sp}     
    \vspace*{1em}
  \end{subfigure}
  \begin{subfigure}[b]{0.21\textwidth}
    \centering
    \includegraphics[height=10.75em]{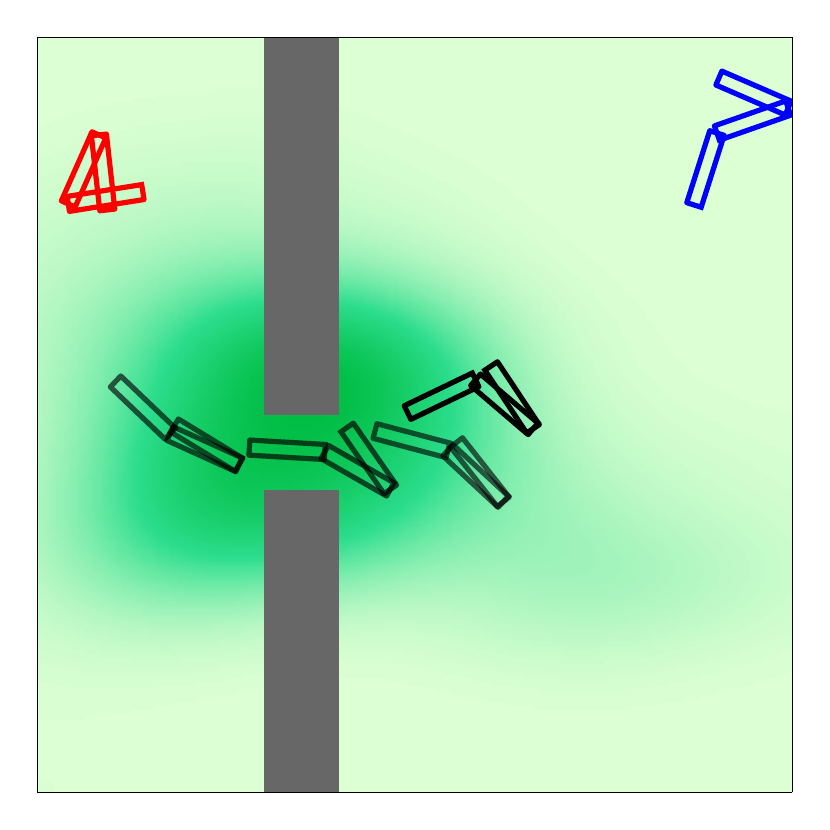}
    % \framebox[\linewidth]{\raisebox{0pt}[0.7\linewidth][0pt]{{\large Snake}}}
    \caption{}
    \label{fig:4_3D_lego}     
    \vspace*{1em}
  \end{subfigure}
%%%%%%%%%%%%%%%%%%%%%%%%%%%%%%% 9D SNAKE
  % \begin{subfigure}[b]{0.27\textwidth}
  %   \centering
  %   % \framebox[\linewidth]{\raisebox{0pt}[0.7\linewidth][0pt]{{\large Snake}}}
  %   \includegraphics[height=10.70em]{fig4/fig4_e}
  %   \caption{}
  %   \label{fig:4_7D_sr}
  %   \vspace*{1em}
  % \end{subfigure}
  % \begin{subfigure}[b]{0.27\textwidth}
  %   \centering
  %   % \framebox[\linewidth]{\raisebox{0pt}[0.7\linewidth][0pt]{{\large Snake}}}
  %   \includegraphics[height=10.70em]{fig4/fig4_f}
  %   \caption{}
  %   \label{fig:4_7D_pl}
  %   \vspace*{1em}
  % \end{subfigure}
  % \begin{subfigure}[b]{0.21\textwidth}
  %   \centering
  %   \includegraphics[height=10.75em]{fig_snake/SP_3L}
  %   % \framebox[\linewidth]{\raisebox{0pt}[0.7\linewidth][0pt]{{\large Snake}}}
  %   \caption{}
  %   \label{fig:4_7D_sp}     
  %   \vspace*{1em}
  % \end{subfigure}
  % \begin{subfigure}[b]{0.21\textwidth}
  %   \centering
  %   \includegraphics[height=10.75em]{fig_snake/LEGO_3L}
  %   % \framebox[\linewidth]{\raisebox{0pt}[0.7\linewidth][0pt]{{\large Snake}}}
  %   \caption{}
  %   \label{fig:4_7D_lego}     
  %   \vspace*{1em}
  % \end{subfigure}
%%%%%%%%%%%%%%%%%%%%%%%%%%%%%%%
  \begin{subfigure}[b]{0.27\textwidth}
    \centering
    \includegraphics[height=10.75em]{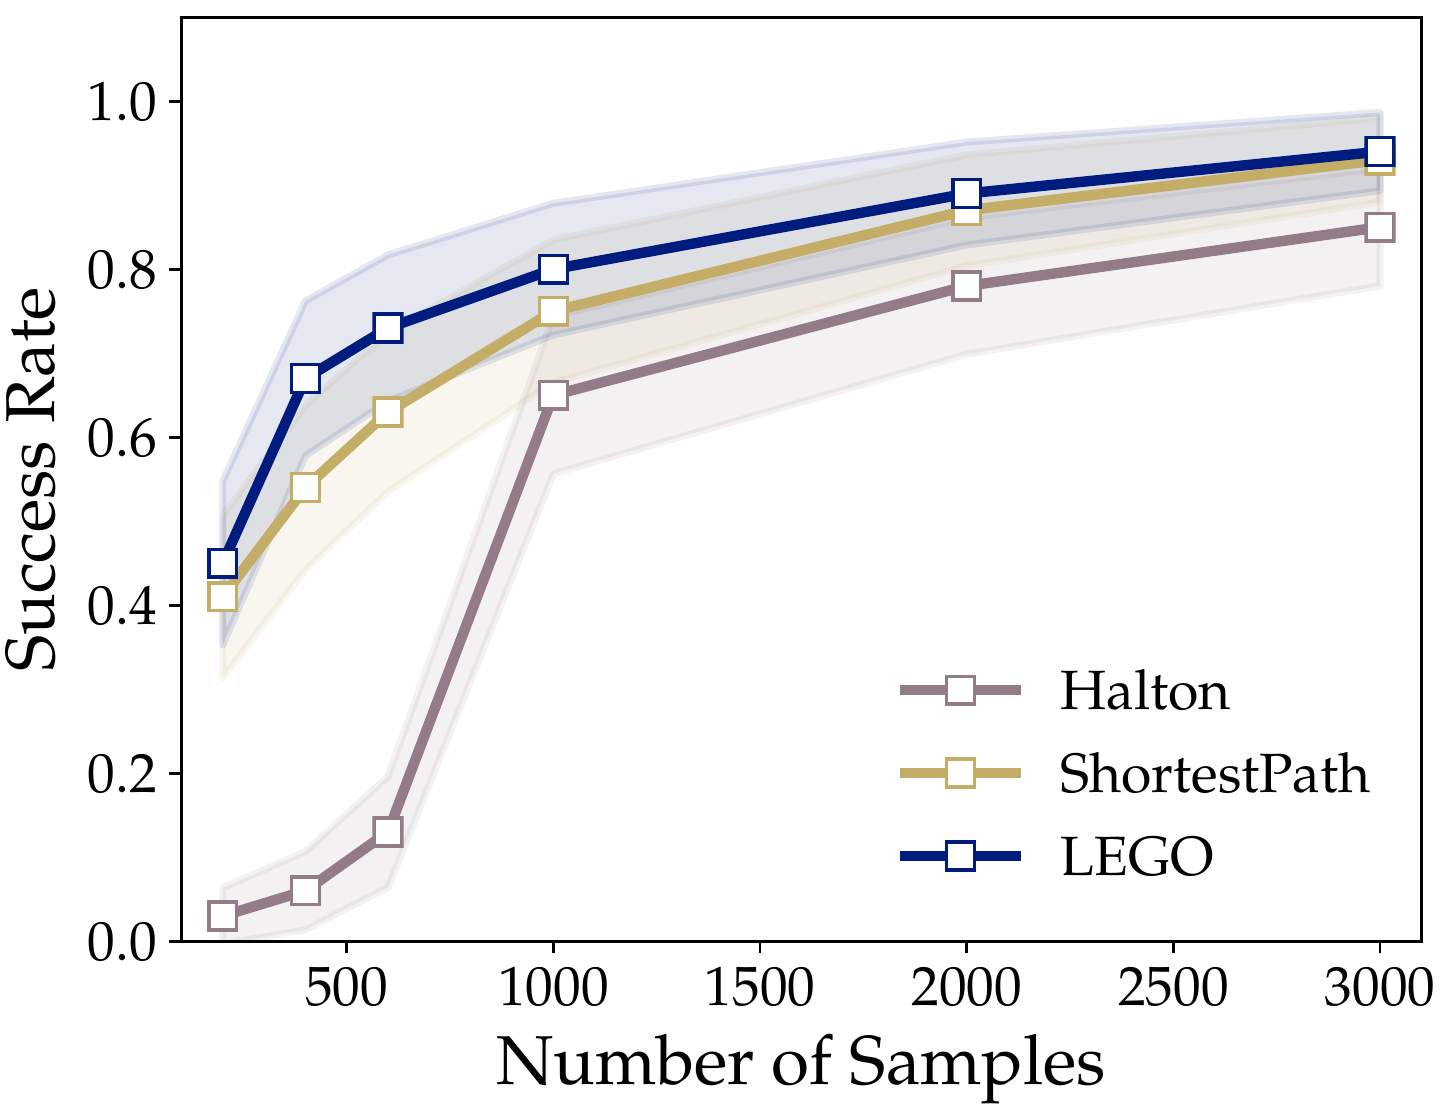}
    \caption{}
    \label{fig:4_herb_sr}
    \vspace*{1em}
  \end{subfigure}
  \begin{subfigure}[b]{0.27\textwidth}
    \centering
    \includegraphics[height=10.75em]{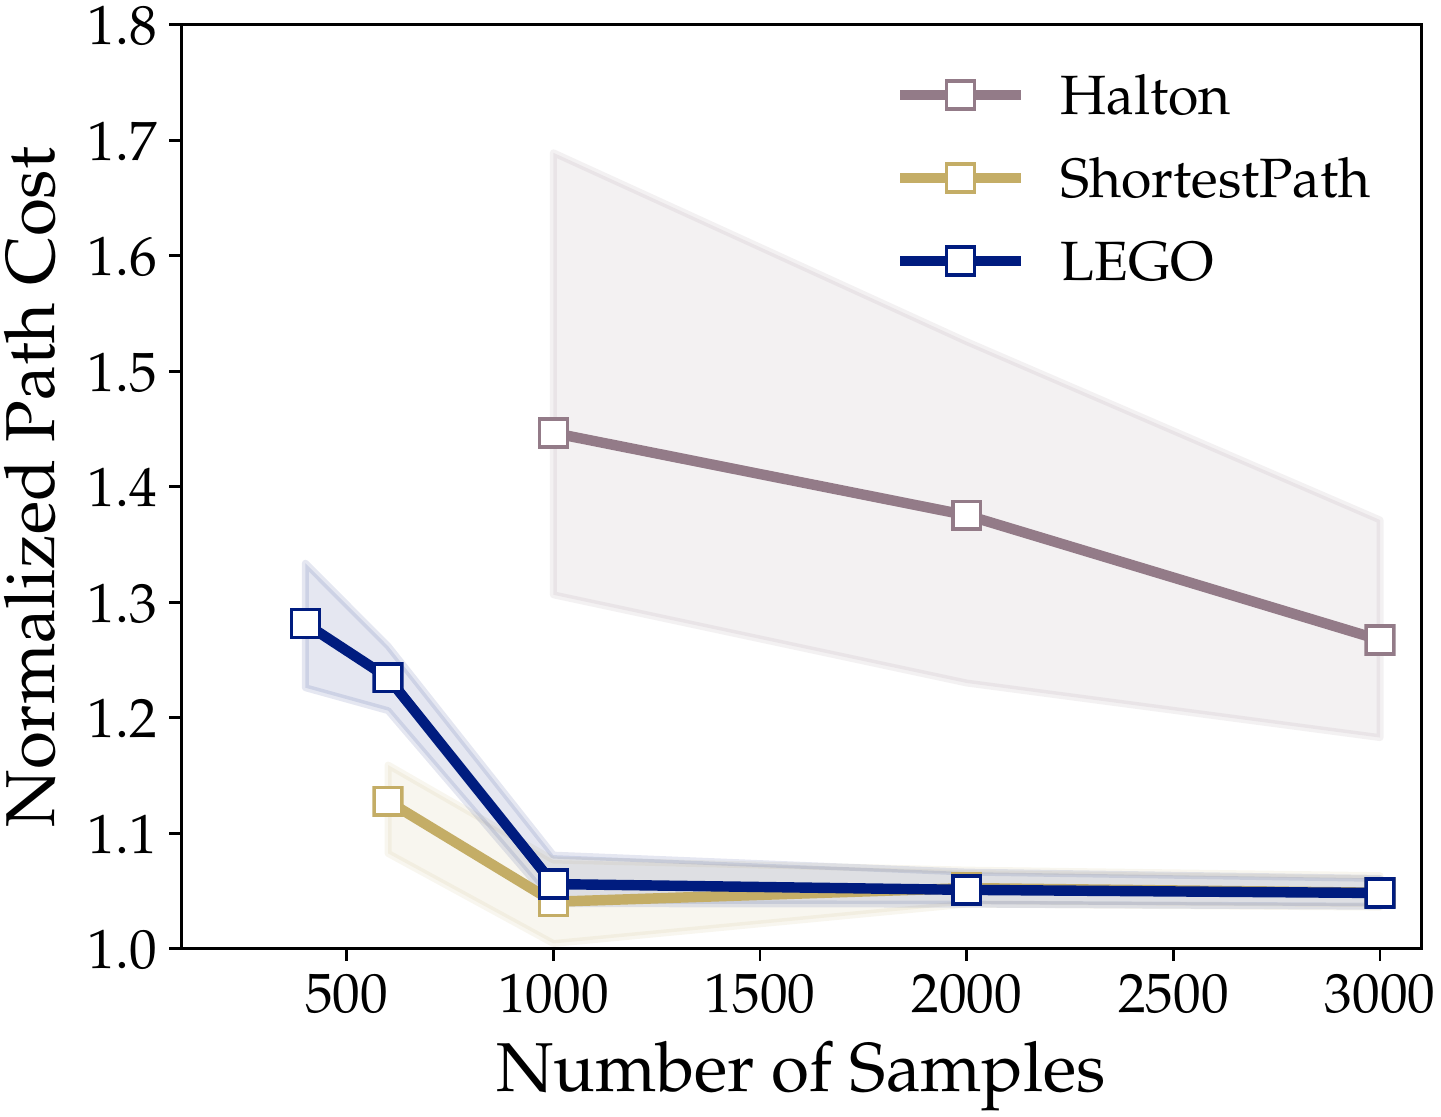}
    \caption{}
    \label{fig:4_herb_pl}     
    \vspace*{1em}
  \end{subfigure}
  \begin{subfigure}[b]{0.21\textwidth}
    \centering
    \includegraphics[trim=50 20 30 0, clip, height=10.75em]{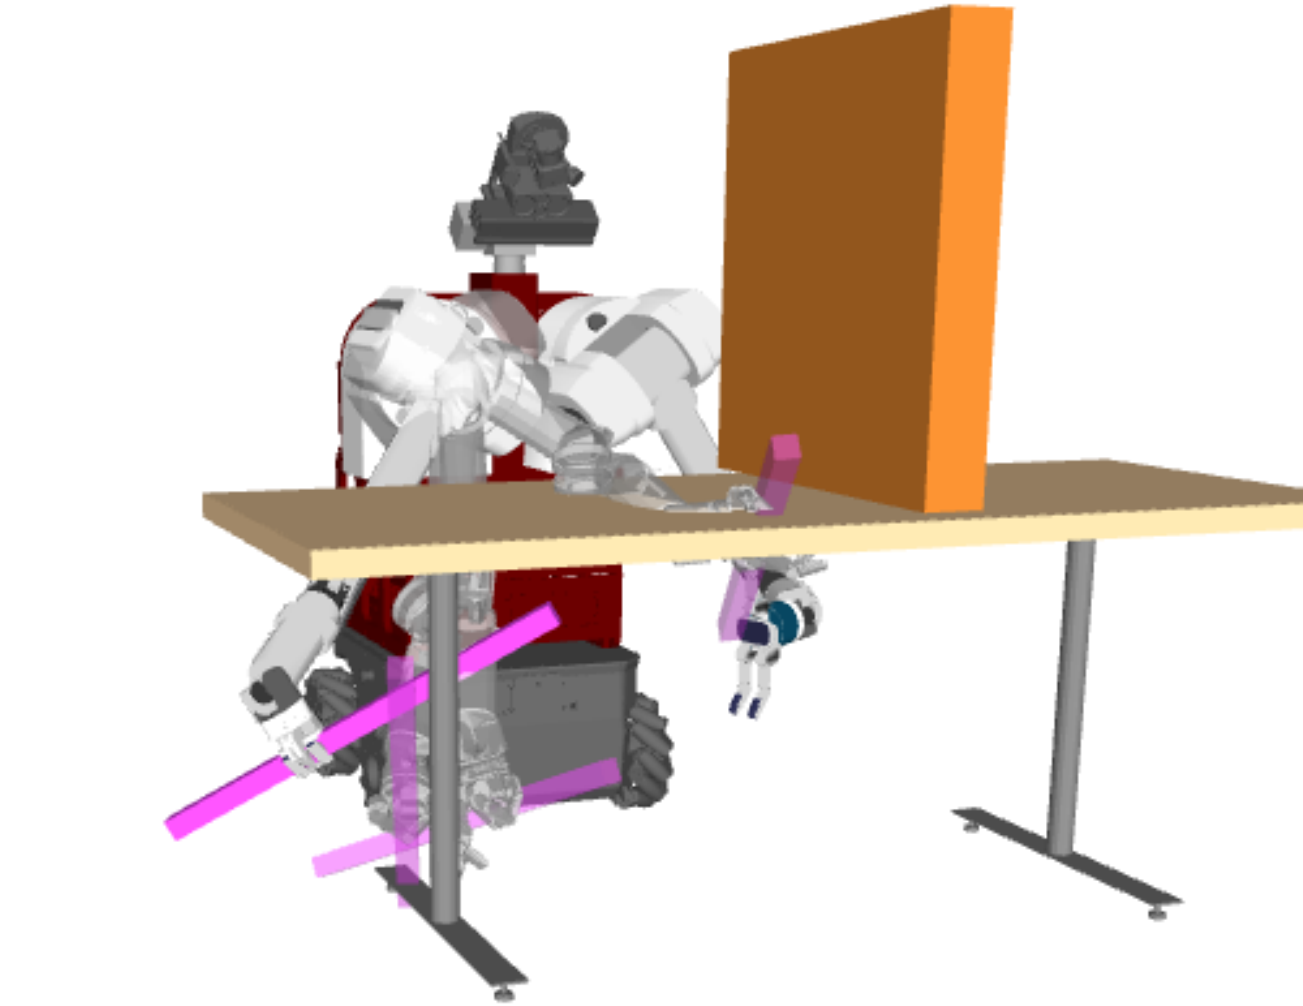}
    \caption{}
    \label{fig:4_herb_sp}     
    \vspace*{1em}
  \end{subfigure}
  \begin{subfigure}[b]{0.21\textwidth}
    \centering
    \includegraphics[trim=0 20 50 0, clip, height=10.75em]{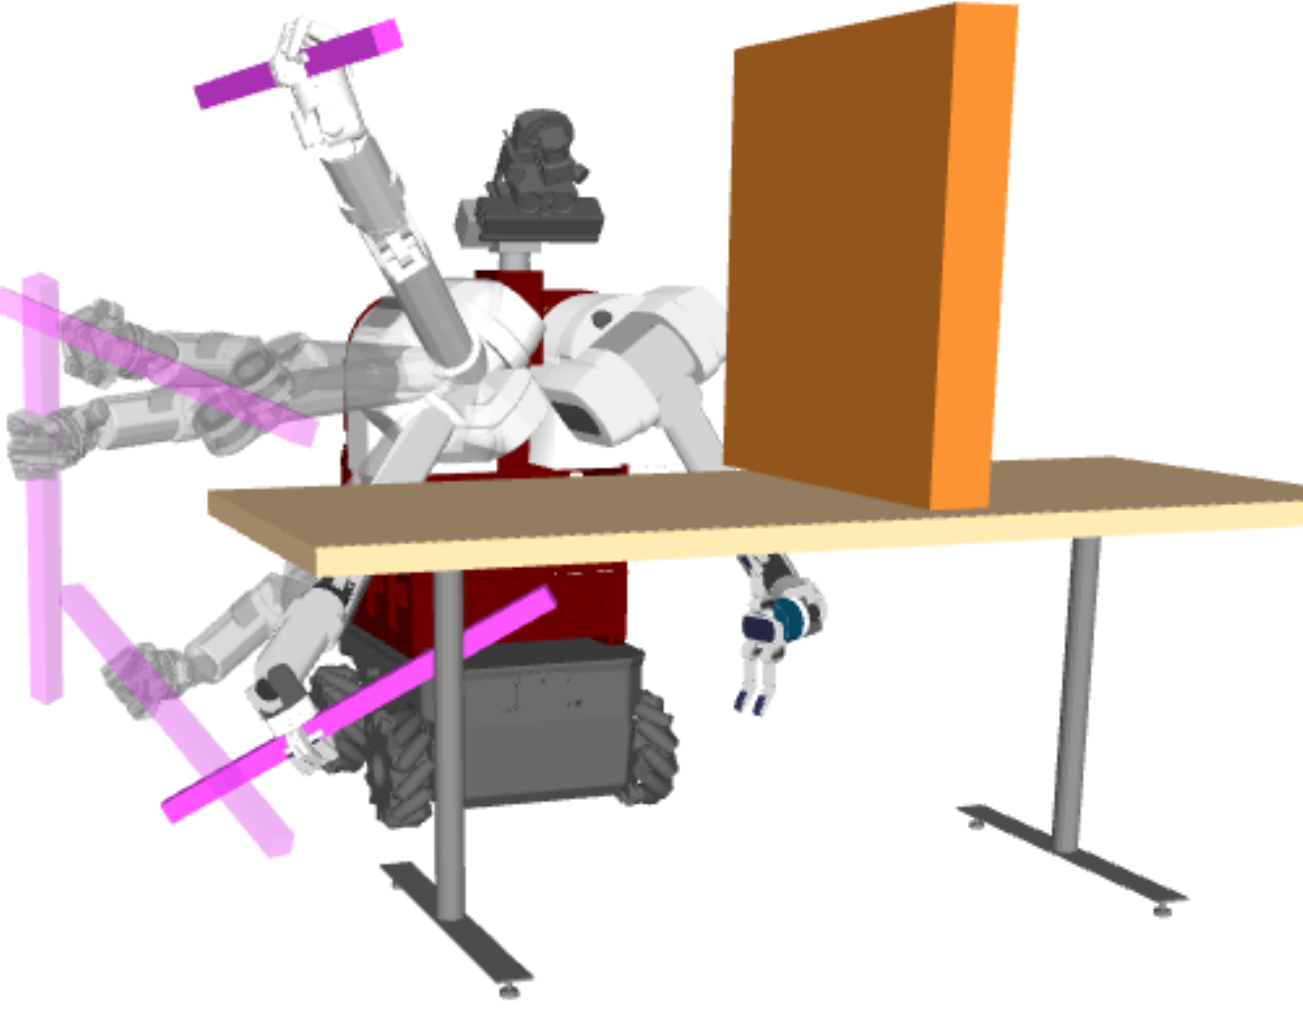}
    \caption{}
    \label{fig:4_herb_lego}
    \vspace*{1em}
  \end{subfigure}
%%%%%%%%%%%%%%%%%%%%%%%%%%%%%%%
\caption{Comparisons of \algSP against \algLEGO. Each row follows pattern (from the left): First figure shows the success rate, second figure shows the normalized path length, third figure shows \algSP and fourth figure shows \algLEGO.}
\label{fig:experiments}
\end{figure*}
